# Supplementary material for: Entropic balance with feedback control: information equalities and tight inequalities
Source: arXiv:2509.15322 ancillary file (2026-02-11)
Supplement: Supplementary file 1 [file SM-RyP25.pdf]

# Supplemental Material for “Entropic balance with feedback control: information equalities and tight inequalities”

N. Ruiz-Pino\* and A. Prados†

*Física Teórica, Multidisciplinary Unit for Energy Science,  
Universidad de Sevilla, Apdo. de Correos 1065, E-41080 Sevilla, Spain*

(Dated: September 18, 2025)

The key features for our study of the Markovian description developed in Ref. [1] are presented in Sec. I. The second law in the Markovian picture, where only the last value of the controller state is considered, is derived in Sec. II. The second law in the chain picture, where the whole chain of control actions is considered, is derived in Sec. III. Equation (10) of the main text, which orders the inequalities for the work in the Markovian and chain descriptions, is proven in Sec. IV. Sections V and VI are devoted to proving Eqs. (11) and (18) of the main text, respectively. Finally, Sec. VII gives details of the numerical simulations and also presents additional numerical results.

## CONTENTS

|                                                           |    |
|-----------------------------------------------------------|----|
| I. Key aspects of the Markovian description               | 1  |
| II. Derivation of the second law in the Markovian picture | 4  |
| III. Derivation of the second law in the chain picture    | 4  |
| IV. Proof of Eq. (10) of the main text                    | 7  |
| V. Proof of Eq. (11) of the main text                     | 8  |
| VI. Proof of Eq. (18) of the main text                    | 10 |
| VII. Numerical simulations: procedure and further results | 11 |
| A. Numerical procedure                                    | 11 |
| B. Additional numerical results                           | 12 |
| References                                                | 14 |

## I. KEY ASPECTS OF THE MARKOVIAN DESCRIPTION

In the time intervals between measurements,  $\tau_{\text{FP}}^{(n)} = (t_{n-1}^+, t_n^-)$ , the joint probability  $P(x, c, t)$  follows the Fokker-Planck equation

$$\partial_t P(x, c, t) = \gamma^{-1} \partial_x [-F(x, c) P(x, c, t) + \beta^{-1} \partial_x P(x, c, t)] \equiv -\partial_x J(x, c, t). \quad (\text{S1})$$

or in terms of operators,

$$\partial_t P(x, c, t) = \hat{\mathcal{L}}^{(c)} P(x, c, t) \equiv -\partial_x J(x, c, t), \quad (\text{S2})$$

where  $F(x, c) = -\partial_x V(x, c) + f \equiv -\partial_x \tilde{V}(x, c)$ . This equation is also fulfilled by the conditional probability distribution function  $P(x|c, t)$ , because  $P(c, t)$  does not vary between measurements.

In the long-time limit, the system approaches a steady state that can be either an equilibrium state or a non-equilibrium steady state; in the former (latter), the steady current vanishes (it is different from zero). To be concrete, let us focus on the one-dimensional case with periodic boundary conditions in the finite interval  $[-L, +L]$ —in the

---

\* nrui1@us.es

† prados@us.es

whole real line  $(-\infty, +\infty)$ ,  $J_s(c) = 0$  due to the boundary conditions at  $\pm\infty$  and the stationary solution of Eq. (S1) is always that of equilibrium for  $\tilde{V}(x, c)$ . For periodic boundary conditions, one has

$$P_s(x|c) = K(c)e^{-\beta\tilde{V}(x,c)} - \beta\gamma J_s(c) \int_{-L}^x dx' e^{-\beta[\tilde{V}(x,c) - \tilde{V}(x',c)]}, \quad \beta\gamma J_s(c) = K(c) \frac{e^{-\beta\tilde{V}(L,c)} - e^{-\beta\tilde{V}(-L,c)}}{\int_{-L}^L dx e^{-\beta[\tilde{V}(L,c) - \tilde{V}(x,c)]}}. \quad (\text{S3})$$

There appear two distinct cases. First,  $f = 0$ , for which  $\tilde{V}(x, c) = V(x, c)$  and the periodicity of  $V(x, c)$ ,  $V(L, c) - V(-L, c) = 0$ , entail that  $J_s(c) = 0$ . Therefore, the stationary solution  $P_s(x|c)$  reduces to the equilibrium distribution,  $P_s(x|c) = e^{-\beta V(x,c)}/Z(c)$ . Second,  $f \neq 0$ , for which  $\tilde{V}(L, c) - \tilde{V}(-L, c) = -2fL \neq 0$  and thus  $J_s(c) \neq 0$ . The external force  $f$  breaks detailed balance and prevents the system from reaching the equilibrium state.

For  $f = 0$ , the propagator of the process  $K(x, t|x', c)$ , i.e. the solution of Eq. (S1) with initial condition  $\delta(x - x')$ , can be analytically computed in terms of the eigenfunctions and eigenvalues of the Fokker-Planck operator  $\hat{\mathcal{L}}^{(c)}$ —which is Hermitian with a scalar product with weight  $1/P_s(x|c)$ . Specifically, one has

$$K(x, t|x', c) = P_s(x|c) + \frac{1}{P_s(x'|c)} \sum_{n=1} \phi_n^{(c)}(x') \phi_n^{(c)}(x) e^{-\lambda_n^{(c)} t}, \quad (\text{S4})$$

where

$$\hat{\mathcal{L}}^{(c)} P_s(x|c) = 0, \quad \hat{\mathcal{L}}^{(c)} \phi_n^{(c)}(x) = -\lambda_n^{(c)} \phi_n^{(c)}(x), \quad \lambda_n^{(c)} > 0 \text{ for } n \geq 1. \quad (\text{S5})$$

Equation (S4) implies the validity of the detailed balance condition [2]

$$K(x, t|x', c) P_s(x'|c) = K(x', t|x, c) P_s(x|c). \quad (\text{S6})$$

Therefore, in the one-dimensional case with periodic boundary conditions, detailed balance holds for  $f = 0$ , whereas it is broken for  $f \neq 0$ . In the whole real line, detailed balance always holds with  $P_s(x|c)$  being given by the equilibrium distribution for  $\tilde{V}(x, c)$ .

At the measurement times  $t_n = n\Delta t_m$ , the control value is updated. Specifically, since we set the value  $c$  with probability  $\Theta(c|x_n^-)$  when the measured state is  $x_n^- \equiv x(t_n^-)$ , we have

$$P(x, c, t_n^+) = \Theta(c|x) P(x, t_n^-) = \Theta(c|x) \sum_{c'} P(x, c', t_n^-) \quad (\text{S7})$$

in the ensemble picture. Note that (i)  $P(x, t)$  is, as expected from a physical point of view, continuous at the measurement:  $P(x, t_n^+) = P(x, t_n^-)$ , (ii)  $\Theta(c|x)$  is thus the conditional probability of the control variable  $c$  for a given system state  $x$  just after the measurement,  $\Theta(c|x) = P(x, c, t_n^+)/P(x, t_n^+)$ . If the system operates in an error-free regime, the domain  $\mathcal{D} \subset \mathbb{R}^d$  in which the system state belongs is split into disjoint subdomains  $\mathcal{X}_c$ , such that  $\cup_c \mathcal{X}_c = \mathcal{D}$ , and  $\Theta(c|x) = \mathbf{1}_c(x)$ , where  $\mathbf{1}_c(x)$  is the indicator function in  $\mathcal{X}_c$ , i.e.  $\mathbf{1}_c(x) = 1$  if  $x \in \mathcal{X}_c$  and zero otherwise. Therefore, each value  $x$  uniquely determines  $c$  with probability one—all other control values are taken with probability zero. Measurement errors can be incorporated as follows. For the sake of simplicity, let us consider again the one-dimensional case. Suppose that the measurement error is  $\Delta x$ , i.e. we only know that the state of the system lies on the interval  $(x - \Delta x/2, x + \Delta x/2)$ . Therein, the probability  $\Theta(c|x)$  is no longer restricted to 0 or 1, being proportional to the length of the interval  $(x - \Delta x/2, x + \Delta x/2)$  in each  $\mathcal{X}_c$ . A specific example of  $\Theta(c|x)$  for different values of  $\Delta x$  is plotted in Fig. 2 of the main text.

The discontinuous change in the joint probability distribution during the infinitesimal measurement interval  $\tau_m^{(n)} = (t_n^-, t_n^+)$  is given by

$$P(x, c, t_n^+) - P(x, c, t_n^-) = \Theta(c|x) \sum_{c' \neq c} P(x, c', t_n^-) - [1 - \Theta(c|x)] P(x, c, t_n^-). \quad (\text{S8})$$

Now, we can write a complete evolution equation for the joint process  $(x, c)$ , valid for all times:

$$\partial_t P(x, c, t) = \hat{\mathcal{L}}^{(c)} P(x, c, t) + \sum_n \hat{W}_n P(x, c, t), \quad (\text{S9})$$

where

$$\hat{W}_n P(x, c, t) \equiv \delta(t - t_n) \Theta(c|x) \underbrace{\sum_{c'} P(x, c', t)}_{P(x, t)} - \delta(t - t_n^-) P(x, c, t). \quad (\text{S10})$$

Equation (S9) is a differential Chapman-Kolmogorov equation [3] for the Markovian joint stochastic process  $(x, c)$ . Its first term  $\hat{\mathcal{L}}^{(c)}P$ , of Fokker-Planck type, provides the continuous evolution of the joint probability distribution during the time intervals  $\tau_{\text{FP}}^{(n)}$ , while its second term  $\sum_n \hat{W}_n P$ , of master equation type, provides the discontinuous evolution of the joint probability distribution at the measurement times  $t_n$ , i.e. during the infinitesimal time interval  $\tau_m^{(n)}$ .

A formal solution of the differential Chapman-Kolmogorov equation (S9) for the joint process  $(x, c)$  can be written. In terms of the propagator  $K(x, t|x', c)$  of the Fokker-Planck equation with  $\hat{\mathcal{L}}^{(c)}$ , we have

$$P(x, c, t) = \int dx' K(x, t - t_{n-1}^+ | x', c) P(x', c, t_{n-1}^+), \quad t \in \tau_{\text{FP}}^{(n)}, \quad (\text{S11})$$

where  $P(x, c, t_{n-1}^+)$  is obtained recursively as

$$P(x, c, t_{n-1}^+) = \Theta(c|x) \underbrace{\sum_{c'} \int dx' K(x, \Delta t_m | x', c') P(x', c', t_{n-2}^+)}_{P(x, t_{n-1}^-)}. \quad (\text{S12})$$

If detailed balance holds for the Fokker-Planck evolution,  $K(x, t|x', c)$  is given by Eq. (S4). If detailed balance does not hold, the operator  $\hat{\mathcal{L}}^{(c)}$  is no longer Hermitian and one needs to obtain both its left and right eigenfunctions [2].

Moreover, it is possible to prove an  $H$ -theorem that ensures that, regardless of the initial conditions, the joint process  $(x, c)$  converges to a long-time periodic state with period  $\Delta t_m$ , which we denote by  $\tilde{P}(x, c, t)$ . This  $H$ -theorem holds independently of having detailed balance or not in the Fokker-Planck evolution. It is over this long-time periodic state  $\tilde{P}(x, c, t)$  that we consider the thermodynamic balance.

Coarse-graining in time, we may define the process  $\vec{x}_n = \{x_0, x_1, \dots, x_n\}$ , which only stores the values of the system state at the measurement times. The dynamics of  $\vec{x}_n$  is Markovian; to be consistent with the notation employed in the main text, we introduce the notation  $P(x_n) \equiv P(x = x_n, t = t_n) = \sum_{c_n} P(x = x_n, c = c_n, t = t_n)$ . The evolution of  $P(x_n)$  is given by a Markov chain:

$$P(x_n) = \int dx_{n-1} P(x_n | x_{n-1}) P(x_{n-1}), \quad P(x_n | x_{n-1}) \equiv \sum_{c_{n-1}} K(x_n, \Delta t_m | x_{n-1}, c_{n-1}) \Theta(c_{n-1} | x_{n-1}). \quad (\text{S13})$$

This equation, which gives the propagator  $P(x_n | x_{n-1})$  of the coarse-grained  $\vec{x}_n$  process in terms of the propagators of the Fokker-Planck equation for each potential  $V(x, c)$ , is equivalent to Eq. (52b) of Ref. [1]. Note that  $x$  is not Markovian over the fine time scale  $t$ : the control value  $c$  is needed to have the time evolution of  $x$  for all times. It is only over the “rougher” timescale  $t_n$  that the system state becomes a Markov process, specifically a Markov chain in discrete time  $t_n = n\Delta t_m$ . This Markov chain has a stationary solution, which we denote by  $P_M$ , that is approached for  $n \gg 1$ .

This stationary state over the coarse-grained timescale makes it possible to construct the long-time periodic solution  $\tilde{P}(x, c, t)$ —guaranteed by the  $H$ -theorem—over the fine timescale  $t$ . Since  $P(x, t)$  is continuous at the measurements, for long times we have  $P(x, t_n^-) = P_M(x)$  and then  $P(x, c, t_n^+) = \Theta(c|x) P_M(x)$ , i.e.

$$\tilde{P}(x, c, t) = \int dx' K(x, t - t_{n-1}^+ | x', c) \Theta(c|x') P_M(x'), \quad t \in \tau_{\text{FP}}^{(n)}. \quad (\text{S14})$$

Although  $x$  is Markovian on the coarse-grained scale,  $c$  is not; it is not possible to obtain a closed evolution equation for  $P(c)$  over the coarse-grained timescale of measurement times. However, the marginal distribution of the control variable  $P(c, t)$  reaches a steady value in the long-time limit: due to the periodicity of the joint distribution  $\tilde{P}(x, c, t)$ , the corresponding marginal distribution  $\tilde{P}(c, t)$  verifies  $\tilde{P}(c, t_n^-) = \tilde{P}(c, t_{n+1}^-)$ . Moreover,  $\tilde{P}(c, t_{n+1}^-) = \tilde{P}(c, t_n^+)$ , because both  $t_n^+$  and  $t_{n+1}^-$  belong in the interval  $\tau_{\text{FP}}^{(n+1)}$ , where the control variable is fixed. Putting together these equalities,  $\tilde{P}(c, t_n^-) = \tilde{P}(c, t_n^+)$ , i.e.  $\tilde{P}$  does not vary at the measurements, and thus we can drop the time dependence in  $\tilde{P}$  and write  $\tilde{P}(c, t) = P_s(c)$ .

In the next sections, consistently with the notation used in the main text, we drop the tilde and denote the long-time periodic joint probability by  $P(x, c, t)$ , and the corresponding marginal distributions by  $P(x, t)$  and  $P_s(c)$ .

## II. DERIVATION OF THE SECOND LAW IN THE MARKOVIAN PICTURE

During the time interval  $\tau_{\text{FP}}^{(n)}$ , we have

$$\begin{aligned}
\dot{S}_{xc} &= - \sum_c \int dx \partial_t P(x, c, t) \ln P(x, c, t) = \sum_c \int dx \partial_x J(x, c, t) \ln P(x, c, t) = - \sum_c \int dx J(x, c, t) \partial_x \ln P(x, c, t) \\
&= - \sum_c \int dx \frac{J(x, c, t)}{P(x, c, t)} [-\gamma\beta J(x, c, t) + \beta F(x, c) P(x, c, t)] = \underbrace{\gamma\beta \sum_c \int dx \frac{J^2(x, c, t)}{P(x, c, t)}}_{\equiv \sigma_{xc}^{\text{FP}}} - \underbrace{\beta \sum_c \int dx F(x, c) J(x, c, t)}_{= -\langle \dot{Q} \rangle} \\
&= \sigma_{xc} + \beta \langle \dot{Q} \rangle.
\end{aligned} \tag{S15}$$

Integrating this equation over the whole interval  $\tau_{\text{FP}}^{(n)}$  gives  $\Delta S_{xc, \text{FP}}$  in Eq. (3) of the main text.

Let us now consider the Markovian entropy change at the measurement:

$$\Delta_{\text{m}} S_{xc} \equiv S_{xc}^+ - S_{xc}^- = - \sum_c \int dx P(x, c, t_n^+) \ln P(x, c, t_n^+) + \sum_c \int dx P(x, c, t_n^-) \ln P(x, c, t_n^-). \tag{S16}$$

The mutual information between the system and controls states after and before the measurement is

$$I_{\pm} \equiv \sum_c \int dx P(x, c, t_n^{\pm}) \ln \frac{P(x, c, t_n^{\pm})}{P(x, t_n) P_s(c)} = -S_{xc}(t_n^{\pm}) + S_x(t_n) + S_c, \tag{S17}$$

where

$$S_x(t) \equiv - \int dx P(x, t) \ln P(x, t), \quad S_c \equiv - \sum_c P_s(c) \ln P_s(c), \tag{S18}$$

are the entropies of the marginal (non-Markovian) processes  $x$  and  $c$ , respectively. Recall that  $P(x, t)$  is continuous at the measurement; this is the reason why we have written  $P(x, t_n)$  instead of  $P(x, t_n^{\pm})$ . The mutual information change at the measurement is thus

$$\Delta_{\text{m}} I \equiv I_+ - I_- = -\Delta_{\text{m}} S_{xc} + \Delta_{\text{m}} S_x \overset{0}{\rightarrow} + \Delta_{\text{m}} S_c \overset{0}{\rightarrow}, \tag{S19}$$

which is equivalent to the expression for  $\Delta_{\text{m}} S_{xc}$  in Eq. (3) of the main text, because  $S_{xc}(t) = S_c + S_{x|c}(t)$ . Both  $\Delta_{\text{m}} S_x$  and  $\Delta_{\text{m}} S_c$  vanish: the former because  $P(x, t)$  is always continuous at the measurement times, the latter because it is time-independent in the long-time regime we are considering.

## III. DERIVATION OF THE SECOND LAW IN THE CHAIN PICTURE

In the literature, e.g. see Refs. [4–7], the whole chain of control actions  $\vec{c}_{n-1} \equiv \{c_0, c_1, \dots, c_{n-1}\}$  up to a time  $t \in \tau_{\text{FP}}^{(n)}$  is kept by the observer. In the chain picture, a Fokker-Planck equation analogous to Eq. (S1) also governs the time evolution of  $P(x, \vec{c}_n, t)$ :

$$\partial_t P(x, \vec{c}_{n-1}, t) = \gamma^{-1} \partial_x [-F(x, c_{n-1}) P(x, \vec{c}_{n-1}, t) + k_B T \partial_x P(x, \vec{c}_{n-1}, t)] \equiv -\partial_x J(x, \vec{c}_{n-1}, t), \quad t \in \tau_{\text{FP}}^{(n)} = (t_{n-1}^+, t_n^-). \tag{S20}$$

The Markovian probability density and current are related to  $P(x, \vec{c}_n, t)$  and  $J(x, \vec{c}_n, t)$  by

$$P(x, c_{n-1}, t) = \sum_{\vec{c}_{n-2}} P(x, \vec{c}_{n-1}, t), \quad J(x, c_{n-1}, t) = \sum_{\vec{c}_{n-2}} J(x, \vec{c}_{n-1}, t), \quad t \in \tau_{\text{FP}}^{(n)}. \tag{S21}$$

The conditional probability  $P(x|\vec{c}_{n-1}, t)$  also obeys a Fokker-Planck equation analogous to Eq. (S20), with its corresponding conditional current  $J(x|\vec{c}_{n-1}, t)$ , because

$$P(x|\vec{c}_{n-1}, t) = \frac{P(x, \vec{c}_{n-1}, t)}{P(\vec{c}_{n-1})}, \quad J(x|\vec{c}_{n-1}, t) = \frac{J(x, \vec{c}_{n-1}, t)}{P(\vec{c}_{n-1})}, \quad t \in \tau_{\text{FP}}^{(n)}. \tag{S22}$$

We write  $P(\vec{c}_{n-1})$  instead of  $P(\vec{c}_{n-1}, t)$  to stress that it has the same value for all times in the interval  $\tau_{\text{FP}}^{(n)}$ . Yet, it changes when there is a measurement at one of the times  $t_n = n\Delta t_m$ ; thereat, the size of the chain of control actions varies discontinuously from  $\vec{c}_{n-1}$  to  $\vec{c}_n$ .

On the one hand, the energy balance is identical in the Markovian and chain descriptions:

$$\sum_{\vec{c}_{n-1}} \int dx V(x, c_{n-1}) P(x, \vec{c}_{n-1}, t) = \sum_{c_{n-1}} \int dx V(x, c_{n-1}) P(x, c_{n-1}, t) = \langle V \rangle(t), \quad (\text{S23a})$$

$$\int_{t_{n-1}^+}^{t_n^-} dt \sum_{\vec{c}_{n-1}} \int dx f J(x, \vec{c}_{n-1}, t) = \int_{t_{n-1}^+}^{t_n^-} dt \sum_{c_{n-1}} \int dx f J(x, c_{n-1}, t) = \langle W_{\text{FP}} \rangle, \quad (\text{S23b})$$

$$\int_{t_{n-1}^+}^{t_n^-} dt \sum_{\vec{c}_{n-1}} \int dx F(x, c_{n-1}) J(x, \vec{c}_{n-1}, t) = \int_{t_{n-1}^+}^{t_n^-} dt \sum_{c_{n-1}} \int dx F(x, c_{n-1}) J(x, c_{n-1}, t) = \langle Q \rangle, \quad (\text{S23c})$$

$$\begin{aligned} & \sum_{\vec{c}_n} \int dx V(x, c_n) P(x, \vec{c}_n, t_n^+) - \sum_{\vec{c}_{n-1}} \int dx V(x, c_{n-1}) P(x, \vec{c}_{n-1}, t_n^-) \\ &= \sum_{c_n} \int dx V(x, c_n) P(x, c_n, t_n^+) - \sum_{c_{n-1}} \int dx V(x, c_{n-1}) P(x, c_{n-1}, t_n^-) = \langle W_{\text{m}} \rangle, \end{aligned} \quad (\text{S23d})$$

where we have repeatedly made use of Eq. (S21).

On the other hand, the entropy balance is different. We start from the entropy of the system plus the controller in the chain description, i.e.

$$S_{x\vec{c}}(t) \equiv \sum_{\vec{c}_{n-1}} \int dx P(x, \vec{c}_{n-1}, t) \ln P(x, \vec{c}_{n-1}, t) = S_{\vec{c}}(t) + S_{x|\vec{c}}(t), \quad t \in \tau_{\text{FP}}^{(n)}, \quad (\text{S24})$$

where the entropy of the chain of control actions  $S_{\vec{c}}$  and the entropy of the particle  $S_{x|\vec{c}}$  in this description are

$$S_{\vec{c}}(t) = - \sum_{\vec{c}_{n-1}} P(\vec{c}_{n-1}) \ln P(\vec{c}_{n-1}), \quad S_{x|\vec{c}}(t) = - \sum_{\vec{c}_{n-1}} P(\vec{c}_{n-1}) \int dx P(x|\vec{c}_{n-1}, t) \ln P(x|\vec{c}_{n-1}, t), \quad t \in \tau_{\text{FP}}^{(n)}. \quad (\text{S25})$$

In the chain description,  $P(x, \vec{c}_{n-1}, t)$  is not periodic due to the increasing size of  $\vec{c}_{n-1}$ —and the entropy of the chain of control actions is not constant but increases monotonically [4, 8]. Therefore, neither is it equivalent to analyse the dynamics of  $S_{x\vec{c}}$  and  $S_{x|\vec{c}}$  nor to carry out the entropy balance over  $k$  cycles and one cycle. In order to compare the results in the chain description with those in the Markovian description, we need to consider the average value over many cycles of the entropy change of the particle:

$$\overline{\Delta S_{x|\vec{c}}} \equiv \lim_{k \rightarrow \infty} k^{-1} \sum_{n=1}^k \Delta^{(n)} S_{x|\vec{c}} \equiv \lim_{k \rightarrow \infty} k^{-1} \sum_{n=1}^k (\Delta_{\text{FP}}^{(n)} S_{x|\vec{c}} + \Delta_{\text{m}}^{(n)} S_{x|\vec{c}}). \quad (\text{S26})$$

An analogous notation was introduced in Eq. (9) of the main text for the average over many cycles of the transfer entropy.

Between measurements, the entropy variation in the chain description can be derived by using the Fokker-Planck

equation (S20) for  $P(x|\vec{c}_n, t)$ . Then we have, for  $t \in \tau_{\text{FP}}^{(n)}$ ,

$$\begin{aligned} \dot{S}_{x|\vec{c}} &= - \sum_{\vec{c}_{n-1}} P(\vec{c}_{n-1}) \int dx \partial_t P(x|\vec{c}_{n-1}, t) \ln P(x|\vec{c}_{n-1}, t) = \sum_{\vec{c}_{n-1}} P(\vec{c}_{n-1}) \int dx \partial_x J(x|\vec{c}_{n-1}, t) \ln P(x|\vec{c}_{n-1}, t) \\ &= - \sum_{\vec{c}_{n-1}} P(\vec{c}_{n-1}) \int dx J(x|\vec{c}_{n-1}, t) \partial_x \ln P(x|\vec{c}_{n-1}, t) \end{aligned} \quad (\text{S27})$$

$$\begin{aligned} &= - \sum_{\vec{c}_{n-1}} P(\vec{c}_{n-1}) \int dx \frac{J(x|\vec{c}_{n-1}, t)}{P(x|\vec{c}_{n-1}, t)} [-\gamma\beta J(x|\vec{c}_{n-1}, t) + \beta F(x, c_{n-1}) P(x|\vec{c}_{n-1}, t)] \\ &= \gamma\beta \sum_{\vec{c}_{n-1}} P(\vec{c}_{n-1}) \int dx \frac{J^2(x|\vec{c}_{n-1}, t)}{P(x|\vec{c}_{n-1}, t)} - \beta \sum_{\vec{c}_{n-1}} P(\vec{c}_{n-1}) \int dx F(x, c_{n-1}) J(x|\vec{c}_{n-1}, t) \\ &= \underbrace{\gamma\beta \sum_{\vec{c}_{n-1}} \int dx \frac{J^2(x, \vec{c}_{n-1}, t)}{P(x, \vec{c}_{n-1}, t)}}_{\equiv \sigma_{x\vec{c}}^{(n)}} - \underbrace{\beta \sum_{\vec{c}_{n-1}} \int dx F(x, c_{n-1}) J(x, \vec{c}_{n-1}, t)}_{= -\langle \dot{Q} \rangle} = \sigma_{x\vec{c}}^{(n)} + \beta \langle \dot{Q} \rangle. \end{aligned} \quad (\text{S28})$$

Therefore, we have

$$\Delta_{\text{FP}}^{(n)} S_{x|\vec{c}} = \Sigma_{x\vec{c}}^{(n)} + \beta \langle Q \rangle, \quad (\text{S29})$$

where  $\Sigma_{x\vec{c}}^{(n)}$  is the entropy production in the chain description in the time interval  $\tau_{\text{FP}}^{(n)}$ :

$$\Sigma_{x\vec{c}}^{(n)} = \int_{t_{n-1}^+}^{t_n^-} dt \sigma_{x\vec{c}}^{(n)} = \gamma\beta \int_{t_{n-1}^+}^{t_n^-} dt \sum_{\vec{c}_{n-1}} \int dx \frac{J^2(x, \vec{c}_{n-1}, t)}{P(x, \vec{c}_{n-1}, t)} \geq 0, \quad (\text{S30})$$

At the measurement, the entropy of the control varies due to the increase of the chain size:

$$\Delta_{\text{m}}^{(n)} S_{\vec{c}} \equiv S_{\vec{c}}(t_n^+) - S_{\vec{c}}(t_n^-) = - \sum_{\vec{c}_n} P(\vec{c}_n) \ln P(\vec{c}_n) + \sum_{\vec{c}_{n-1}} P(\vec{c}_{n-1}) \ln P(\vec{c}_{n-1}) = - \sum_{\vec{c}_n} P(\vec{c}_n) \ln \frac{P(\vec{c}_n)}{P(\vec{c}_{n-1})} \equiv \mathcal{I}_{\vec{c}}^{(n)}, \quad (\text{S31})$$

where  $\mathcal{I}_{\vec{c}}^{(n)}$  is the transfer entropy of the chain of control actions at the  $n$ -th measurement,

$$\mathcal{I}_{\vec{c}}^{(n)} \equiv - \sum_{\vec{c}_n} P(\vec{c}_n) \ln \frac{P(\vec{c}_n)}{P(\vec{c}_{n-1})} = - \sum_{\vec{c}_n} P(\vec{c}_n) \ln P(c_n|\vec{c}_{n-1}) \geq 0. \quad (\text{S32})$$

Since the entropy of the system plus the controller is continuous at the measurements [1],

$$\Delta_{\text{m}} S_{x|\vec{c}}^{(n)} \equiv S_{x|\vec{c}}(t_n^+) - S_{x|\vec{c}}(t_n^-) = -\Delta_{\text{m}}^{(n)} S_{\vec{c}} = -\mathcal{I}_{\vec{c}}^{(n)} \leq 0. \quad (\text{S33})$$

Let us consider the entropy variation in the chain picture over  $k$  cycles,

$$S_{x|\vec{c}}(t_k^+) - S_{x|\vec{c}}(t_0^+) = \sum_{n=1}^k \Delta S_{x|\vec{c}}^{(n)} = \sum_{n=1}^k [\Delta_{\text{FP}}^{(n)} S_{x|\vec{c}} + \Delta_{\text{m}}^{(n)} S_{x|\vec{c}}] = \sum_{n=1}^k [\Sigma_{x\vec{c}}^{(n)} - \mathcal{I}_{\vec{c}}^{(n)}] + k\beta \langle Q \rangle, \quad (\text{S34})$$

i.e.

$$\lim_{k \rightarrow \infty} k^{-1} [S_{x|\vec{c}}(t_k^+) - S_{x|\vec{c}}(t_0^+)] = \overline{\Sigma_{x\vec{c}}} - \overline{\mathcal{I}_{\vec{c}}} + \beta \langle Q \rangle. \quad (\text{S35})$$

The first term vanishes:  $S_{x|\vec{c}}(t_k^+)$  remains bounded because the entropy diminishes when increasing the conditioning [9], and the length of the chain of control actions increases without limit. Therefore, bringing to bear the first principle,  $\langle Q \rangle = -\langle W \rangle$ , we have

$$\beta \langle W \rangle = \overline{\Sigma_{x\vec{c}}} - \overline{\mathcal{I}_{\vec{c}}} \geq -\overline{\mathcal{I}_{\vec{c}}} \quad (\text{S36})$$

In this way, we have reobtained the bound for  $\langle W \rangle$  in the literature [4–7].

Note that calculating  $\mathcal{I}_{\vec{c}}$  involves the calculation of the entropy of a very long chain of control actions, since

$$\overline{\mathcal{I}_{\vec{c}}} = \lim_{k \rightarrow \infty} k^{-1} \sum_{n=1}^k \mathcal{I}_{\vec{c}}^{(n)} = \lim_{k \rightarrow \infty} \sum_{\vec{c}_k} \frac{-P(\vec{c}_k) \ln P(\vec{c}_k)}{k} + \lim_{k \rightarrow \infty} \frac{\sum_{c_0} P(c_0) \ln P(c_0)}{k}. \quad (\text{S37})$$

As a consequence, the evaluation of  $\mathcal{I}_{\vec{c}}$  is challenging, both from an analytical and a numerical perspective, when there are correlations between the  $c_n$ 's. This is the reason why the application of inequality (S36) has often been restricted to situations in which these correlations disappear and  $P(\vec{c}_k) = \prod_{n=1}^k P(c_n)$  [6, 7, 10].

The bound in Eq. (S36) can be improved by splitting the entropy production in the chain description into positive-definite housekeeping and excess parts,  $\Sigma_{x\vec{c}}^{(n)} = \Sigma_{x\vec{c}}^{\text{hk},(n)} + \Sigma_{x\vec{c}}^{\text{ex},(n)}$  [7], with

$$\Sigma_{x\vec{c}}^{\text{hk},(n)} \equiv \gamma\beta \int_{t_{n-1}^+}^{t_n^-} dt \sum_{\vec{c}_{n-1}} \int dx \frac{J_s^2(x, \vec{c}_{n-1})}{P_s^2(x, \vec{c}_{n-1})} P(x, \vec{c}_{n-1}, t), \quad (\text{S38})$$

$$\Sigma_{x\vec{c}}^{\text{ex},(n)} \equiv \gamma\beta \int_{t_{n-1}^+}^{t_n^-} dt \sum_c \int dx \left[ \frac{J(x, \vec{c}_{n-1}, t)}{P(x, \vec{c}_{n-1}, t)} - \frac{J_s(x, \vec{c}_{n-1})}{P_s(x, \vec{c}_{n-1})} \right]^2 P(x, \vec{c}_{n-1}, t), \quad (\text{S39})$$

where  $P_s(x, \vec{c}_{n-1})$  is the stationary solution in the time interval  $\tau_{\text{FP}}^{(n)}$  of the Fokker-Planck equation for  $P(x, \vec{c}_{n-1}, t)$ , Eq. (S20), and  $J_s(x, \vec{c}_{n-1})$  the corresponding current. We have kept the  $x$ -dependence in  $J_s$  because in the  $d$ -dimensional case,  $\partial_x J_s(x, \vec{c}_{n-1})$  must be understood as the divergence of  $J_s$ . For  $d = 1$ ,  $J_s$  becomes independent of  $x$ .

Interestingly, the housekeeping contribution to the entropy production in the chain picture is equal to that in the Markovian one, i.e.  $\Sigma_{x\vec{c}}^{(n),\text{hk}} = \Sigma_{xc}^{\text{hk}}$ . In our framework, there is only one stationary solution of the Fokker-Planck equation for each potential  $V(x, c)$ , i.e.  $P_s(x|c)$  is unique. Since  $P_s(x, \vec{c}_n)$  obeys the same equation as  $P_s(x, c_{n-1}) = P_s(c_{n-1})P_s(x|c_{n-1})$ , we conclude that

$$P_s(x, \vec{c}_{n-1}) = a(\vec{c}_{n-1}) P_s(x, c_{n-1}), \quad (\text{S40})$$

where  $a(\vec{c}_{n-1})$  is an arbitrary function of the chain  $\vec{c}_n$ . This implies that

$$J_s(x, \vec{c}_{n-1}) = a(\vec{c}_{n-1}) J_s(x, c_{n-1}) \implies \frac{J_s(x, \vec{c}_{n-1})}{P_s(x, \vec{c}_{n-1})} = \frac{J_s(x, c_{n-1})}{P_s(x, c_{n-1})} = \frac{J_s(x|c_{n-1})}{P_s(x|c_{n-1})}, \quad (\text{S41})$$

and  $P_s(x, \vec{c}_{n-1})$  is indeed stationary,  $\partial_x J_s(x, \vec{c}_{n-1}) = a(\vec{c}_{n-1}) \partial_x J_s(x, c_{n-1}) = 0$ . Therefore,

$$\Sigma_{x\vec{c}}^{\text{hk},(n)} \equiv \gamma\beta \int_{t_{n-1}^+}^{t_n^-} dt \sum_{\vec{c}_{n-1}} \int dx \frac{J_s^2(x|c_{n-1})}{P_s^2(x|c_{n-1})} P(x, \vec{c}_{n-1}, t) = \gamma\beta \int_{t_{n-1}^+}^{t_n^-} dt \sum_{c_{n-1}} \int dx \frac{J_s^2(x|c_{n-1})}{P_s^2(x|c_{n-1})} \underbrace{\sum_{\vec{c}_{n-2}} P(x, \vec{c}_{n-1}, t)}_{P(x, c_{n-1}, t)} = \Sigma_{xc}^{\text{hk}}, \quad (\text{S42})$$

where we have taken into account Eq. (6a) of the main text; note that  $\Sigma_{xc}^{\text{hk}}$  is independent of  $n$ . The equality between  $\Sigma_{x\vec{c}}^{\text{hk}}$  and  $\Sigma_{xc}^{\text{hk}}$  is sensible from a physical point of view, since the housekeeping heat is directly related to the housekeeping contribution of the entropy production,  $\langle Q^{\text{hk}} \rangle = T \Sigma_{xc}^{\text{hk}}$  [11–13].

Bringing to bear the splitting of the entropy production, the bound in Eq. (S36) can thus be refined to [7]

$$\beta \langle W \rangle = \Sigma_{xc}^{\text{hk}} + \overline{\Sigma_{x\vec{c}}^{\text{ex}}} - \overline{\mathcal{I}_{\vec{c}}} \geq \Sigma_{xc}^{\text{hk}} - \overline{\mathcal{I}_{\vec{c}}} \geq -\overline{\mathcal{I}_{\vec{c}}}, \quad (\text{S43})$$

which is precisely inequality (8) in the main text.

#### IV. PROOF OF EQ. (10) OF THE MAIN TEXT

The Markovian inequalities are always tighter than their chain counterparts because entropy production in the Markovian description is always smaller than in the chain description. Let us prove it by defining a scalar product in the chain description as

$$\langle u|v \rangle \equiv \sum_{\vec{c}_{n-1}} \frac{u(\vec{c}_n)v(\vec{c}_n)}{P(x, \vec{c}_n, t)}, \quad t \in \tau_{\text{FP}}^{(n+1)}; \quad (\text{S44})$$

note that  $\vec{c}_n = \{\vec{c}_{n-1}, c_n\}$ , so that the resulting scalar depends on  $c_n$ . Choosing  $u(\vec{c}_n) = J(x, \vec{c}_n, t)$  and  $v(\vec{c}_n) = P(x, \vec{c}_n, t)$  and making use of the Cauchy-Schwarz inequality,

$$\left( \sum_{\vec{c}_{n-1}} J(x, \vec{c}_n, t) \right)^2 \leq \sum_{\vec{c}_{n-1}} \frac{J^2(x, \vec{c}_n, t)}{P(x, \vec{c}_n, t)} \sum_{\vec{c}_{n-1}} P(x, \vec{c}_n, t), \quad (\text{S45})$$

i.e.

$$\frac{J^2(x, c_n, t)}{P(x, c_n, t)} \leq \sum_{\vec{c}_{n-1}} \frac{J^2(x, \vec{c}_n, t)}{P(x, \vec{c}_n, t)} \quad (\text{S46})$$

$$\frac{J^2(x, c_n, t)}{P(x, c_n, t)} \leq \sum_{\vec{c}_{n-1}} \frac{J^2(x, \vec{c}_{n-1}, c_n, t)}{P(x, \vec{c}_{n-1}, c_n, t)}, \quad (\text{S47})$$

where we have made use of Eq. (S21). The above equation immediately implies

$$\Sigma_{xc} \leq \Sigma_{x\vec{c}}^{(n)}, \forall n \implies \Sigma_{xc} \leq \overline{\Sigma_{x\vec{c}}} \implies \Delta_m I \leq \overline{\mathcal{I}_{\vec{c}}}, \quad (\text{S48})$$

because the work in a cycle  $\langle W \rangle$  is the same in both descriptions—as proven in Sec. III of this Supplemental Material. Note that the above proof remains valid for  $d$  dimensions, interpreting  $J^2$  as the modulus of the vector  $J$ , since inequality (S46) holds for every component thereof. Equation (S48) immediately implies the ordered inequalities in Eq. (10) of the main text.

## V. PROOF OF EQ. (11) OF THE MAIN TEXT

In the formalism used in Ref. [10], a key quantity is the transfer entropy of the chain of measurements  $\vec{x}_k$  up to time  $t_k$ :

$$\langle \mathcal{I}_{\vec{x}} \rangle = \lim_{k \rightarrow \infty} k^{-1} \sum_{n=1}^k \mathcal{I}_{\vec{x}}^{(n)}, \quad (\text{S49a})$$

$$\begin{aligned} \mathcal{I}_{\vec{x}}^{(n)} &\equiv -\langle \ln P(x_n | \vec{x}_{n-1}) \rangle = -\int d\vec{x}_n P(\vec{x}_n) \ln P(x_n | \vec{x}_{n-1}) = -\int d\vec{x}_n P(\vec{x}_n) \ln P(x_n | x_{n-1}) \\ &= -\int dx_{n-1} \int dx_n P(x_{n-1}, x_n) \ln P(x_n | x_{n-1}). \end{aligned} \quad (\text{S49b})$$

In the last step, we have brought to bear that the chain  $\vec{x}_n$  is a Markov process, as discussed in Sec. I, and integrated over  $\{x_0, \dots, x_{n-2}\}$ . Then, we can write for arbitrary  $\Delta t_m$ :

$$\mathcal{I}_{\vec{x}}^{(n)} = -\sum_{c_{n-1}} \int dx_{n-1} \int dx_n P(x_{n-1}, c_{n-1}, x_n) \ln P(x_n | x_{n-1}). \quad (\text{S50})$$

For error-free measurement,  $c_{n-1}$  is enslaved to  $x_{n-1}$ , and  $P(x_{n-1}, c_{n-1}, x_n)$  vanishes if  $x_{n-1} \notin \mathcal{X}_{c_{n-1}}$ ;

$$\begin{aligned} P(x_{n-1}, c_{n-1}, x_n) &= P(x_n | x_{n-1}, c_{n-1}) P(x_{n-1}, c_{n-1}) = P(x_n | x_{n-1}, c_{n-1}) P(c_{n-1} | x_{n-1}) P(x_{n-1}) \\ &= P(x_n | x_{n-1}, c_{n-1}) P(x_{n-1}) \mathbf{1}_{c_{n-1}}(x_{n-1}). \end{aligned} \quad (\text{S51})$$

Now, we make use of Eq. (S13) for the propagator  $P(x_n | x_{n-1})$  of the coarse-grained  $\vec{x}_n$  process in terms of the propagators of the Fokker-Planck equation for each potential  $V(x, c)$ . In the error-free case,  $\Theta(c_{n-1} | x_{n-1}) = \mathbf{1}_{c_{n-1}}(x_{n-1})$ , i.e.  $\Theta(c_{n-1} | x_{n-1}) = 1$  if  $x_{n-1} \in \mathcal{X}_{c_{n-1}}$ , and zero otherwise. Therefore,

$$P(x_n | x_{n-1}) = \sum_{c_{n-1}} K(x_n, \Delta t_m | x_{n-1}, c_{n-1}) \mathbf{1}_{c_{n-1}}(x_{n-1}) \implies P(x_n | x_{n-1}) = K(x_n, \Delta t_m | x_{n-1}, c_{n-1}) \text{ if } x_{n-1} \in \mathcal{X}_{c_{n-1}}, \quad (\text{S52})$$



i.e. where the integrand of (S50) does not vanish. This implies that

$$\mathcal{I}_{\vec{x}}^{(n)} = - \sum_{c_{n-1}} \int dx_{n-1} \int dx_n P(x_{n-1}, c_{n-1}, x_n) \ln K(x_n, \Delta t_m | x_{n-1}, c_{n-1}), \quad (\text{S53})$$

which entails that  $\mathcal{I}_{\vec{x}}^{(n)}$  is independent of  $n$  in the long time regime we are analysing.

Now we investigate the unavailable information  $I_u$ , by considering the reverse process described in the main text. Specifically, one has

$$\langle \mathcal{I}_u \rangle = \lim_{k \rightarrow \infty} k^{-1} \sum_{n=1}^k \mathcal{I}_u^{(n)} \quad (\text{S54})$$

$$\mathcal{I}_u^{(n)} = - \langle \ln P^R(x_n^R | \vec{x}_{n-1}^R) \rangle = - \sum_{n=1}^k \int d\vec{x}_k P(\vec{x}_k) \ln P^R(x_n^R | \vec{x}_{n-1}^R) \quad (\text{S55})$$

Above,  $P^R$  denotes the probability of observing the reverse trajectory considered under the application of the reverse chain of control actions  $\vec{c}_k^R$ .

The reverse process, carried out under the fixed chain of control actions determined in the forward process, is also clearly Markovian:  $P^R(x_n^R | \vec{x}_{n-1}^R) = P^R(x_n^R | x_{n-1}^R)$ . To go from  $x_{n-1}^R = x_{k-n+1}$  to  $x_n^R = x_{k-n}$ , the system moves under the action of the potential  $V(x, c_n^R) = V(x, c_{k-n})$ —the one determined in the forward process for the time interval  $\tau_{\text{FP}}^{(k-n+1)} = (t_{k-n}^+, t_{k-n+1}^-)$ . Consistently with the main text, we define  $\tilde{n} = k - n$ . We keep the superscript  $R$  in  $P^R(x_{\tilde{n}} | x_{\tilde{n}+1}; c_{\tilde{n}})$  to stress the fact that the evolution from  $x_{\tilde{n}+1}$  to  $x_{\tilde{n}}$  is done with the value of the control  $c_{\tilde{n}}$ —if it were the forward process, where the value of the control is determined by the measurement of  $x$  at the initial time, the value of the control would have been  $c_{\tilde{n}+1}$ . Integrating over all the variables different from  $\{x_{k-n+1}, x_{k-n}\} = \{x_{\tilde{n}}, x_{\tilde{n}+1}\}$ , we get

$$\mathcal{I}_u^{(n)} = - \int d\vec{x}_k P(\vec{x}_k) \ln P^R(x_n^R | x_{n-1}^R) = - \int dx_{\tilde{n}} dx_{\tilde{n}+1} P(x_{\tilde{n}}, x_{\tilde{n}+1}) \ln P^R(x_{\tilde{n}} | x_{\tilde{n}+1}). \quad (\text{S56})$$

Analogously to what we have done for  $\mathcal{I}_{\vec{x}}^{(n)}$ , we have for arbitrary  $\Delta t_m$  that

$$\mathcal{I}_u^{(n)} = - \sum_{c_{\tilde{n}}} \int dx_{\tilde{n}} dx_{\tilde{n}+1} P(x_{\tilde{n}}, c_{\tilde{n}}, x_{\tilde{n}+1}) \ln P^R(x_{\tilde{n}} | x_{\tilde{n}+1}). \quad (\text{S57})$$

In addition, (i)  $P(x_{\tilde{n}}, c_{\tilde{n}}, x_{\tilde{n}+1}) \neq 0$  only for  $x_{\tilde{n}} \in \mathcal{X}_{c_{\tilde{n}}}$ , and (ii)  $P^R(x_{\tilde{n}} | x_{\tilde{n}+1}) = K(x_{\tilde{n}}, \Delta t_m | x_{\tilde{n}+1}, c_{\tilde{n}})$  if  $x_{\tilde{n}} \in \mathcal{X}_{c_{\tilde{n}}}$ . Then, we write

$$\mathcal{I}_u^{(n)} = - \sum_{c_{\tilde{n}}} \int dx_{\tilde{n}} dx_{\tilde{n}+1} P(x_{\tilde{n}}, c_{\tilde{n}}, x_{\tilde{n}+1}) \ln K(x_{\tilde{n}}, \Delta t_m | x_{\tilde{n}+1}, c_{\tilde{n}}), \quad (\text{S58})$$

which is also independent of  $\tilde{n}$  in the long time regime.

Due to the independence of Eqs. (S53) and (S58) of the “time” index  $n$ , we can put them together by changing  $n$  to  $n+1$  in the former and renaming  $\tilde{n}$  to  $n$  in the latter:

$$\mathcal{I}_u^{(n)} - \mathcal{I}_{\vec{x}}^{(n)} = \sum_{c_n} \int dx_n \int dx_{n+1} P(x_n, c_n, x_{n+1}) \ln \frac{K(x_{n+1}, \Delta t_m | x_n, c_n)}{K(x_n, \Delta t_m | x_{n+1}, c_n)}, \quad (\text{S59})$$

For  $f = 0$ , detailed balance holds and

$$K(x_{n+1}, \Delta t_m | x_n, c_n) P_s(x_n, c_n) = K(x_n, \Delta t_m | x_{n+1}, c_n) P_s(x_{n+1}, c_n), \quad (\text{S60})$$

where

$$P_s(x|c) = \frac{e^{-\beta V(x,c)}}{Z(c)}, \quad Z(c) = \int dx e^{-\beta V(x,c)}, \quad f = 0. \quad (\text{S61})$$

Then we have

$$\begin{aligned}
\mathcal{I}_u^{(n)} - \mathcal{I}_{\vec{x}}^{(n)} &= \sum_{c_n} \int dx_n \int dx_{n+1} P(x_n, c_n, x_{n+1}) \ln \frac{P_s(x_{n+1}|c_n)}{P_s(x_n|c_n)}, \\
&= \beta \sum_{c_n} \int dx_n \int dx_{n+1} P(x_n, c_n, x_{n+1}) [V(x_n, c_n) - V(x_{n+1}, c_n)] \\
&= \beta \left[ \sum_{c_n} \int dx_n P(x_n, c_n) V(x_n, c_n) - \sum_{c_n} \int dx_n P(x_{n+1}, c_n) V(x_{n+1}, c_n) \right]. \tag{S62}
\end{aligned}$$

The pair  $\{x_n, c_n\}$  corresponds to time  $t_n^+$ , while the pair  $\{x_{n+1}, c_n\}$  corresponds to time  $t_{n+1}^-$ . Therefore, we have

$$\mathcal{I}_u^{(n)} - \mathcal{I}_{\vec{x}}^{(n)} = \langle V \rangle^+ - \langle V \rangle^- = \beta \langle W \rangle, \tag{S63}$$

which is Eq. (11) of the main text.

## VI. PROOF OF EQ. (18) OF THE MAIN TEXT

The equality between  $\beta \langle W \rangle$  and the quantity  $\overline{\mathcal{I}_u} - \overline{\mathcal{I}_{\vec{x}}}$  can be generalised by including the housekeeping entropy  $\Sigma_{xc}^{\text{hk}}$  to situations in which  $f \neq 0$ , i.e. to cases in which the FP dynamics has a nonequilibrium stationary state with an associated flux  $J_s(x, c) \neq 0$ . In this case, the work has two contributions,

$$\langle W \rangle \equiv \langle W_m \rangle + \langle W_{\text{FP}} \rangle = \sum_c \int dx V(x, c) [P(x, c, t_n^+) - P(x, c, t_n^-)] + \int_{t_{n-1}^+}^{t_n^-} dt \sum_c \int dx f J(x, c, t). \tag{S64}$$

In the non-equilibrium case with  $f \neq 0$ , detailed balance does not hold and the proof of the previous section, valid  $\forall \Delta t_m$ , ceases to be valid. Yet, we can make progress in the non-equilibrium case by considering the limit  $\Delta t_m \rightarrow \infty$ : therein, the propagators of the FP equation tend to the non-equilibrium stationary distribution. Therefore, making use of Eqs.(S50) and (S57), we get

$$\overline{\mathcal{I}_{\vec{x}}} = - \sum_{c_{n-1}} \int dx_{n-1} \int dx_n P(x_{n-1}, c_{n-1}, x_n) \ln P_s(x_n|c_{n-1}) = - \sum_{c_{n-1}} \int dx_n P(c_{n-1}, x_n) \ln P_s(x_n|c_{n-1}), \tag{S65}$$

$$\overline{\mathcal{I}_u} = - \sum_{c_n} \int dx_n \int dx_{n+1} P(x_n, c_n, x_{n+1}) \ln P_s(x_{n+1}|c_n) = - \sum_{c_n} \int dx_n P(x_n, c_n) \ln P_s(x_n|c_n). \tag{S66}$$

As already done in the previous section, we identify pairs  $\{x_n, c_n\}$  and  $\{x_n, c_{n-1}\}$  as corresponding to times  $t_n^+$  and  $t_n^-$ , respectively. Due to the periodicity of the long-time regime, we can shift  $t_n^+ \rightarrow t_{n-1}^+$  to write

$$\overline{\mathcal{I}_u} - \overline{\mathcal{I}_{\vec{x}}} = \sum_c \int dx [P(x, c, t_n^-) - P(x, c, t_{n-1}^+)] \ln P_s(x|c) = \sum_c \int dx \int_{t_{n-1}^+}^{t_n^-} dt \partial_t P(x, c, t) \ln P_s(x|c). \tag{S67}$$

Now we make use of the FP equation and integrate by parts,

$$\overline{\mathcal{I}_u} - \overline{\mathcal{I}_{\vec{x}}} = - \sum_c \int dx \int_{t_{n-1}^+}^{t_n^-} dt \partial_x J(x, c, t) \ln P_s(x|c) = \sum_c \int dx \int_{t_{n-1}^+}^{t_n^-} dt J(x, c, t) \partial_x \ln P_s(x|c). \tag{S68}$$

The housekeeping entropy production  $\Sigma_{xc}^{\text{hk}}$  is given by Eq. (6a) of the main text, which is equivalent to

$$\begin{aligned}
\Sigma_{xc}^{\text{hk}} &= \gamma \beta \sum_c \int dx \int_{t_{n-1}^+}^{t_n^-} dt \frac{J_s(x|c)}{P_s(x|c)} J(x, c, t) = \beta \sum_c \int dx \int_{t_{n-1}^+}^{t_n^-} dt [-\partial_x V(x, c) + f - \beta^{-1} \partial_x \ln P_s(x|c)] J(x, c, t) \\
&= -\beta \sum_c \int dx \int_{t_{n-1}^+}^{t_n^-} dt \partial_x V(x, c) J(x, c, t) + \beta \langle W_{\text{FP}} \rangle - (\overline{\mathcal{I}_u} - \overline{\mathcal{I}_{\vec{x}}}). \tag{S69}
\end{aligned}$$

The first term on the rhs can be integrated by parts once more,

$$\begin{aligned} \sum_c \int dx \int_{t_{n-1}^+}^{t_n^-} dt \partial_x V(x, c) J(x, c, t) &= - \sum_c \int dx V(x, c) \int_{t_{n-1}^+}^{t_n^-} dt \partial_x J(x, c, t) = \sum_c \int dx V(x, c) \int_{t_{n-1}^+}^{t_n^-} dt \partial_t P(x, c, t) \\ &= \langle V \rangle^- - \langle V \rangle^+ = - \langle W_m \rangle. \end{aligned} \quad (S70)$$

Then, we finally write

$$\Sigma_{xc}^{\text{hk}} = \beta \langle W_m \rangle + \beta \langle W_{\text{FP}} \rangle - (\overline{\mathcal{I}_u} - \overline{\mathcal{I}_x}), \quad (S71)$$

i.e.

$$\Sigma_{xc}^{\text{hk}} + \overline{\mathcal{I}_u} - \overline{\mathcal{I}_x} = \beta \langle W \rangle, \quad (S72)$$

which is Eq. (18) of the main text.

## VII. NUMERICAL SIMULATIONS: PROCEDURE AND FURTHER RESULTS

### A. Numerical procedure

As described in the main text, we consider an overdamped Brownian particle in contact with a thermal bath at temperature  $T$  and subject to a fluctuating potential

$$V(x, c) = -c V_0 |x|, \quad c = \pm 1, \quad (S73)$$

to illustrate our theoretical results in a model information engine. The control parameter  $c$  is updated at each measurement time according to a protocol  $\Theta(c|x)$  designed to maximise the work extracted at the measurement, as shown in Fig. 2 of the main text. This control update is done at regularly spaced times  $t = n\Delta t_m$ , each time interval of length  $\Delta t_m$  is termed a cycle.

In our simulations, we have done  $N_{\text{sim}} = 10^5$  realisations of the stochastic process. After a transitory regime with  $n_R$  cycles, the system reaches the periodic long-time state and we reset the time origin, i.e. we set  $n \rightarrow n - n_R$  and  $t \rightarrow t - n_R \Delta t_m$ , and start to store the simulation data for the thermodynamic balance. In this way,  $n = 0$  and  $t = 0$  already corresponds to the long-time regime and we perform  $k$  cycles, i.e. we let the system evolve up to a time  $t = k \Delta t_m$ .

Each cycle comprises two parts. The first part corresponds to the measurement of the particle position at time  $t_n$ , and the subsequent update of the control variable. The last particle position from the previous cycle is identified with  $x(t_n^-) = x_n$ , and the value of the control variable at time  $t_n^+$  is chosen with probability  $\Theta(c_n|x_n)$ . We recall that  $\Theta(c_n|x_n)$  may include errors in the measurement with some precision  $\Delta x$ , as illustrated in the right panel of Fig. 2 of the main text. The second part of the cycle corresponds to the Fokker-Planck evolution between times  $t_n^+$  and  $t_{n+1}^-$ . The simulation of the Fokker-Planck dynamics is carried out by numerically integrating the corresponding Langevin equation with the Euler algorithm,

$$x(t + \Delta t) = x(t) + \gamma^{-1} [-c_n V_0 \text{sgn}(x) + f] \Delta t + z \sqrt{2D\Delta t}, \quad t_n < t < t_{n+1}, \quad (S74)$$

with periodic boundary conditions in the interval  $[-L, L]$ . Dimensionless variables have been used throughout all the numerics, by choosing units as detailed in the main text:  $L$  as the length unit,  $T$  as the energy unit—recall that we have taken  $k_B = 1$ , and  $L^2/D = L^2\gamma/T$  as the time unit. That is, in the simulations we take  $L = 1$ ,  $T = 1$  and  $\gamma = 1$ .

In order to compare with the numerical simulations, theoretical results for the probability distributions have also been obtained by employing Eqs. (S12) and (S11). On the one hand, for a precision  $\Delta x$  in the measurement, the conditional probability  $\Theta(c|x)$  takes the form [1]

$$\Theta(1|x) = \begin{cases} 1, & \text{if } \text{mod}(x - \Delta x, L) < \text{mod}(x + \Delta x, L) \leq L/2, \\ \frac{L/2 - \text{mod}(x - \Delta x, L)}{2\Delta x}, & \text{if } \text{mod}(x - \Delta x, L) \leq L/2 < \text{mod}(x + \Delta x, L), \\ 0, & \text{if } L/2 < \text{mod}(x - \Delta x, L) \leq \text{mod}(x + \Delta x, L), \\ \frac{L/2 + \text{mod}(x + \Delta x, L) - \text{mod}(x - \Delta x, L)}{2\Delta x}, & \text{if } \text{mod}(x + \Delta x, L) \leq L/2 < \text{mod}(x - \Delta x, L), \\ \frac{\text{mod}(x + \Delta x, L)}{2\Delta x}, & \text{if } \text{mod}(x + \Delta x, L) \leq L/2 < \text{mod}(x - \Delta x, L), \\ \frac{L/2}{2\Delta x}, & \text{if } L/2 < \text{mod}(x + \Delta x, L) \leq \text{mod}(x - \Delta x, L). \end{cases} \quad (S75)$$

In order to obtain an easier expression in terms of the modulo function  $\text{mod}(x, L)$ , we have shifted the spatial interval by  $+L$ , i.e. Eq. (S75) has been written for periodic boundary conditions in  $[0, 2L]$ . Once we have specified  $\Theta(1|x)$ , it is straightforward to write  $\Theta(0|x) = 1 - \Theta(1|x)$ . On the other hand, the Fokker-Planck propagator is given by the eigenfunction expansion (S4). For the potentials  $V(x, c)$  in Eq. (S73), one has (i) eigenvalues

$$\lambda_0 = 0, \quad \lambda_n = \frac{\beta F^2}{4} + \frac{n^2 \pi^2}{\beta L^2}, \quad n = 1, \dots, \quad (\text{S76})$$

where we have omitted the  $c$ -dependence, since they are independent  $c$  for the considered potentials, and (ii) eigenfunctions

$$\phi_0^{(c)}(x) = P_s(x|c) = \frac{cF\beta}{2(1 - e^{-F\beta L})} e^{-F\beta|x|}, \quad (\text{S77a})$$

$$\phi_{n,1}^{(c)}(x) = \frac{\sqrt{\phi_0^{(c)}(x)}}{\sqrt{L}} \sin\left(\frac{n\pi x}{L}\right), \quad (\text{S77b})$$

$$\phi_{n,2}^{(c)}(x) = \frac{2\sqrt{\phi_0^{(c)}(x)}}{\sqrt{L\beta\lambda_n^{(c)}}} \left[ \frac{2n\pi}{L} \cos\left(\frac{n\pi x}{L}\right) - cF\beta \sin\left(\frac{n\pi|x|}{L}\right) \right]. \quad (\text{S77c})$$

In all the plots, both in the main text and this Supplemental Material, the infinite expansion in Eq. (S4) has been truncated at  $n = 25$ .

To evaluate the bound on the work that includes the unavailable information,  $\overline{\mathcal{I}_u} - \overline{\mathcal{I}_x}$ , we use the expressions given by Eqs. (S49b) and (S56) and take into account (i) for the propagator of the forward process  $P(x_n|x_{n-1})$  in the coarse-grained timescale of measurement times, Eq. (S13), and (ii) for the corresponding propagator of the reverse process  $P^R(x_{\tilde{n}}|x_{\tilde{n}+1})$ ,

$$P^R(x_{\tilde{n}}|x_{\tilde{n}+1}) = K(x_{\tilde{n}}, \Delta t_m | x_{\tilde{n}+1}, c_{\tilde{n}}^R) \quad (\text{S78})$$

where it has been brought to bear that  $c_{\tilde{n}}^R$  is fixed—thus there is no sum over it, since it was generated in the forward process. Therefore, we have

$$\mathcal{I}_{\tilde{x}}^{(n)} = - \sum_{c_{n-1}} \int dx_{n-1} \int dx_n K(x_n, \Delta t_m | x_{n-1}, c_{n-1}) \Theta(c_{n-1} | x_{n-1}) P_s(x_{n-1}) \ln \left[ \sum_c K(x_n, \Delta t_m | x_{n-1}, c) \Theta(c | x_{n-1}) \right], \quad (\text{S79a})$$

$$\mathcal{I}_u^{(n)} = - \sum_{c_{\tilde{n}}} \int dx_{\tilde{n}} dx_{\tilde{n}+1} K(x_{\tilde{n}+1}, \Delta t_m | x_{\tilde{n}}, c_{\tilde{n}}) \Theta(c_{\tilde{n}} | x_{\tilde{n}}) P_M(x_{\tilde{n}}) \ln K(x_{\tilde{n}}, \Delta t_m | x_{\tilde{n}+1}, c_{\tilde{n}}). \quad (\text{S79b})$$

For error-free measurements.  $\Theta(c|x) = \mathbf{1}_{\mathcal{X}_c}(x)$  and Eqs. (S79a) and (S79b) reduce to Eq. (S53) and (S58), respectively. It is worth stressing that Eqs. (S79a) and (S79b) allow us to compute  $\overline{\mathcal{I}_u} - \overline{\mathcal{I}_x}$  in the presence of measurement errors, making it possible to analyse the behaviour of the corresponding work bound as the error varies across different scenarios.

## B. Additional numerical results

In Fig. 4 of the main text, we have illustrated that the information bound that includes the unavailable information,  $\overline{\mathcal{I}_u} - \overline{\mathcal{I}_x}$ , saturates in the error-free case (left panel), whereas it does not when there is uncertainty in the measurement (right panel). Here, we present further numerical results for the accuracy of this bound as a function of the error in measurement  $\Delta x$  and the time interval between measurements  $\Delta t_m$ . In this context, it is especially relevant to compare this bound with the Markovian one,  $-\Delta_m I$ . This is the purpose of Figs. S1 and S2.

Figure S1 complements the right panel of Fig. 4 of the main text. In this figure, we compare  $\beta \langle W \rangle$  with the unavailable information bound  $\overline{\mathcal{I}_u} - \overline{\mathcal{I}_x}$  and the Markovian bound  $-\Delta_m I$  for different values of the potential parameter  $V_0$ , covering the range from  $V_0 \gg k_B T$  to  $V_0 \ll k_B T$ —the right panel of Fig. 4 of the main text corresponds to the case  $V_0 = 5$ . Note that the interval of  $\Delta x$  shown in each panel is different, to focus on the region where the Markovian bound outperforms the unavailable information's (shaded in grey). Analogously to the case presented in the main text, the interval of  $\Delta x$  where  $\langle W \rangle \geq -\Delta_m I \geq \overline{\mathcal{I}_u} - \overline{\mathcal{I}_x}$  appears in the neighbourhood of the value of  $\Delta x$  at which  $\langle W \rangle$  changes sign.

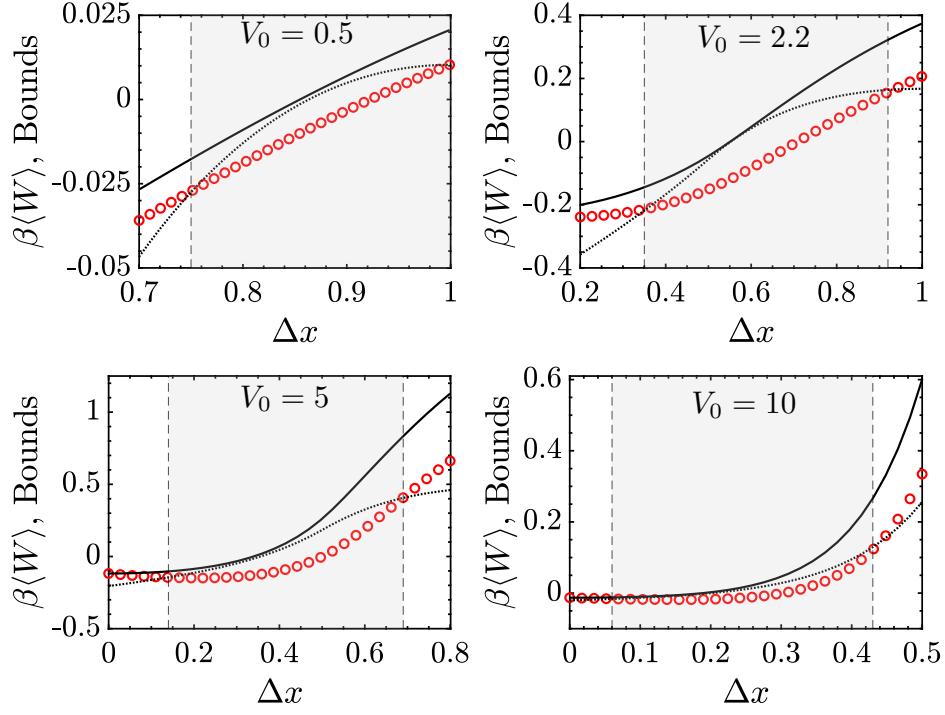

FIG. S1. Average work and bounds as a function of  $\Delta x$  for different values of  $V_0$  (from high to low temperatures). Specifically, the bounds shown are the unavailable information's  $\mathcal{I}_u - \mathcal{I}_x$  (red circles) and the Markovian's  $-\Delta_m I$ . The grey shaded regions correspond to the range of  $\Delta x$  where the Markovian bound is better than the unavailable information bound. All panels corresponds to  $f = 0$  and  $\Delta t_m \rightarrow \infty$ .

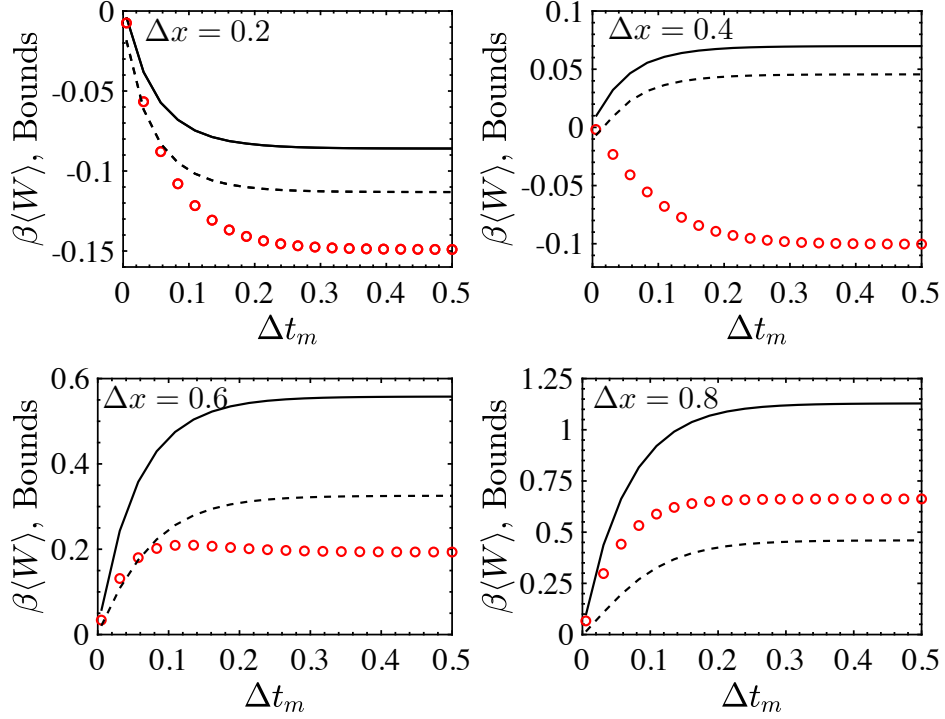

FIG. S2. Average work and bounds as a function of  $\Delta t_m$ , for different values of  $\Delta x$ . The colour and symbol code is the same as in Fig. S1. The Markovian bound outperforms the unavailable information bound for certain values of the measurement error, as already shown in Fig. S1, in particular those at which the sign of the work is reversed—even for finite  $\Delta t_m$ . All panels corresponds to  $f = 0$  and  $V_0 = 5$ .

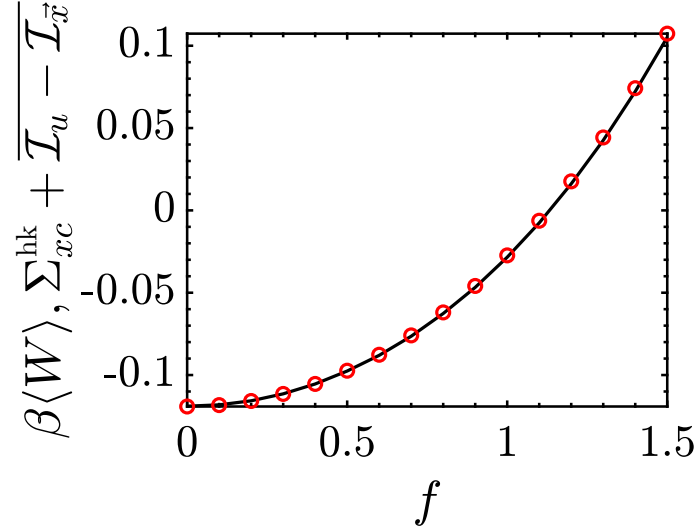

FIG. S3. Numerical check of equality (18) of the main text. Both  $\beta \langle W \rangle$  (solid line) and  $\Sigma_{xc}^{hk} + \overline{\mathcal{I}_u} - \overline{\mathcal{I}_{\vec{x}}}$  (red circles) are plotted as a function of  $f$ , for error-free measurement, i.e.  $\Delta x = 0$ . The plotted data corresponds to  $V_0 = 5$ , with  $\Delta t_m \rightarrow \infty$ .

In Fig. S2,  $\beta \langle W \rangle$  is compared with both bounds as a function of the time interval  $\Delta t_m$  between measurements. This study thus complements that in the previous figure, which corresponded to the limit  $\Delta t_m \rightarrow \infty$ . Each panel presents data for a different value of  $\Delta x$ , as given in the legend. In the first two panels, in which there are regions with both  $\langle W \rangle < 0$  and  $\langle W \rangle > 0$ , the Markovian bound is tighter than the unavailable information's over most of the range of  $\Delta x$ —again, the Markovian information bound is better at estimating the range of values at which the information engine extracts net work from the system.

The two previous figures presented data for  $f = 0$ , in which case the stationary distribution of the Fokker-Planck equation corresponds to equilibrium. Figure S3 shows a numerical test of the equality (18) in the main text for  $f \neq 0$ —in which case the stationary distribution of the Fokker-Planck equation is of non-equilibrium type and detailed balance is broken. Both  $\beta \langle W \rangle$  and  $\Sigma_{xc}^{hk} + \overline{\mathcal{I}_u} - \overline{\mathcal{I}_{\vec{x}}}$  are plotted as a function of the external force  $f$ , with excellent agreement.

- 
- [1] N. Ruiz-Pino and A. Prados, Markovian description of a wide class of feedback-controlled systems: application to the feedback flashing ratchet, *Journal of Statistical Mechanics: Theory and Experiment* **2024**, 083204 (2024).
  - [2] H. Risken, *The Fokker-Planck Equation: Methods of Solution and Applications*, Springer Series in Synergetics (Springer, Berlin Heidelberg, 1996).
  - [3] C. Gardiner, *Stochastic Methods: A Handbook for the Natural and Social Sciences*, Springer Series in Synergetics (Springer Berlin Heidelberg, Berlin - Heidelberg, 2009).
  - [4] F. J. Cao and M. Feito, Thermodynamics of feedback controlled systems, *Physical Review E* **79**, 041118 (2009).
  - [5] J. M. Horowitz and S. Vaikuntanathan, Nonequilibrium detailed fluctuation theorem for repeated discrete feedback, *Physical Review E* **82**, 061120 (2010).
  - [6] T. Sagawa and M. Ueda, Nonequilibrium thermodynamics of feedback control, *Physical Review E* **85**, 021104 (2012).
  - [7] D. Abreu and U. Seifert, Thermodynamics of Genuine Nonequilibrium States under Feedback Control, *Physical Review Letters* **108**, 030601 (2012).
  - [8] N. Ruiz-Pino, D. Villarrubia-Moreno, A. Prados, and F. J. Cao-García, Information in feedback ratchets, *Physical Review E* **108**, 034112 (2023).
  - [9] T. M. Cover and J. A. Thomas, *Elements of information theory*, 2nd ed. (Wiley-Interscience, Hoboken, N.J, 2006) oCLC: ocm59879802.
  - [10] Y. Ashida, K. Funo, Y. Murashita, and M. Ueda, General achievable bound of extractable work under feedback control, *Physical Review E* **90**, 052125 (2014).
  - [11] T. Hatano and S.-i. Sasa, Steady-State Thermodynamics of Langevin Systems, *Physical Review Letters* **86**, 3463 (2001).
  - [12] C. Van den Broeck and M. Esposito, Three faces of the second law. II. Fokker-Planck formulation, *Physical Review E* **82**, 011144 (2010).
  - [13] U. Seifert, Stochastic thermodynamics, fluctuation theorems and molecular machines, *Reports on Progress in Physics* **75**, 126001 (2012).
